# Supplementary material for: Object-Aware Cropping for Self-Supervised Learning
Source: arXiv:2112.00319 source file (2023-04-06)
Supplement: Supplementary file 1 [file appendix.tex]

\appendix

% \section{Appendix}
\section{Details of OpenImages-Subset}
\label{sec:details_openimages}
We show in Fig. \ref{fig:openimages1_distribution}(left) the plot of the number of images and selected class ID's. The mean of the number of images per class is 3762.13. We show additional statistics by removing the classes with more than 10k instances present. We can see this in Fig. \ref{fig:openimages1_distribution}(middle). The mean of number of images per class also comes down from 3762 to 2203. We plot the width and height of all the images present in OpenImages-Subset. We can see from Fig. \ref{fig:openimages1_distribution}(right) that most images are in around $1000 \times 1000$ pixels. with some being significantly larger.

We created OpenImages-Subset by only keeping classes from OpenImages which had at least $900$ images, resulting in a total of $208$ classes with $3762$ images per class on average. For each image in OpenImages-Subset we computed how many images have an extra class that is not present in these $208$ classes: resulting in a very small number $0.002$: mist objects in the subset are from the $208$ classes. The total number of images is $212$k. Finally we computed the number of images with $N$ objects, where $N$ varies from $2$ to $7$. These numbers are: $2/51008; 3/56131; 4/43426; 5/26011; 6/13693; 7/6593$.

{\textbf{Overlap between OHMS and VOC:}
There is a 85\% overlap between OpenImages and VOC, and between COCO and VOC the overlap is 95\%. Between ImageNet and COCO, the overlap is 58\%. Between ImageNet and VOC the overlap is 100\%. Hence the improvements on object detection on VOC is not just because of overlap between the datasets, but because of improved pre-trained features that is learnt by efficient pre-training on OHMS.}
\section{Implementation details for Object localization task}
Let's assume the output of the object proposal method is $X_{o_1}, Y_{o_1}, X_{o_2}, Y_{o_2}$. We firstly feed this object image through random crop operation. The output of the random crop is denoted by  $X_{r_1}, Y_{r_1}, X_{r_2}, Y_{r_2}$. 
% \ashah{I dont think these equations have to be mentioned in the approach part. They are implementation details. I think we need to be crisp in what we are trying to do here; Maybe a figure would help ?}

\begin{align}
X_{f_1} &= \frac{W_f}{W_b} (X_{o_1} + X_{r_1}), ~~
X_{f_2} = \frac{W_f}{W_b} (X_{o_2} + X_{r_2} + W_b/2 )  \\
Y_{f_1} &= \frac{H_f}{H_b}(Y_{o_1} + Y_{r_1})~~, ~~~  
Y_{f_2} = \frac{Y_f}{Y_b}(Y_{o_2} + Y_{r_2} + Y_b/2 ) 
\end{align}
% \begin{eqnarray*}
% % \end{equation}
% X_{f1} &= (X_{o1} + X_{r1}) * W_f / W_b \\   X_{f2} &= (X_{o2} + X_{r2} + W_b/2 ) * W_f / W_b \\
% Y_{f1} &= (Y_{o1} + Y_{r1}) * H_f / H_b \\   Y_{f2} &= (Y_{o2} + Y_{r2} + Y_b/2 ) * Y_f / Y_b
% % \end{equation}
% \end{eqnarray*}
$\frac{W_f}{W_b}$ and $\frac{Y_f}{Y_b}$ are used to scale the cropped image back to the original scale.
So, the new location of the object wrt the original image would be  $X_{f_1}, Y_{f_1}, X_{f_2}, Y_{f_2}$.
% The original image is divided into $p * p$ patches. 
The labels will be set by following condition :
\begin{align}
Y_{ij} = 1  \iff  X_{f_1} < X_{ij} < X_{f_2} \And  Y_{f_1} < Y_{ij} < Y_{f_2} . \\
i,j \in [ {0, 1 * w/p, 2* w/p ... p *w /p} ] . 
\end{align}

\section{Other object proposal methods}
\label{sec:object_proposal_methods}
We also experiment with three object proposal methods, i.e BING \cite{Cheng2014BINGBN}, Edge-Boxes \citep{Zitnick2014EdgeBL} and an unsupervised object proposal method \citep{vo2019unsupervised}. Here we discuss their methodology in more detail.

BING is trained with boxes from Pascal-VOC.
BING \cite{Cheng2014BINGBN} uses the norm of gradients within a fixed window size as a simple feature that is fed into a cascaded SVM framework to make object proposals. This method is trained on the ground-truth bounding boxes of $2501$ images of the PASCAL-VOC \cite{everingham2010pascal} training set. Note that BING does not use any class label, but only label independent bounding box information. BING has the advantage of extremely fast performance (>$125$ fps on an image of size $300 \times 300$), generates many proposals, and generalizes well to many datasets, as shown in \cite{Cheng2014BINGBN} and seen in our empirical results. This makes BING well suited as an object proposal algorithm.

Edge-Boxes \citep{Zitnick2014EdgeBL} is based on a simple heuristic: an object is more likely to be contained in a box if the number of contours wholly inside the box exceed the contours that cross the boundary of the box. In our experiments, we found that EdgeBoxes was slower than BING, although the performance on the generated boxes was similar to that of BING.
%Edge-Boxes produces object proposals using edges present in an image. Their central hypothesis is that the number of contours that are wholly contained in a bounding box is indicative of the likelihood of the box containing an object. They propose a simple box objectness score that measures the number of edges that exist in the box minus those that are members of contours that overlap the box’s boundary. Similar to BING we generate 10 proposals for every image in the OpenImages-Subset and MS-COCO \citep{Lin2014MicrosoftCC} datasets and train on MOCO-V2 and BYOL. EdgeBoxes however is a slower method and doesn't generated as good proposals and final performance on SSL tasks is as poor when compared with BING in our case. So, we mostly focus on BING for our experiments. \\

We also consider an alternative unsupervised object proposal method \citep{vo2019unsupervised}, which uses a robust matching technique that relies on appearance and geometric consistency constraints to assign confidence scores to region proposals. While fully unsupervised, this approach performs similar to BING as shown in Table \ref{tab:voc_moco}, but is significantly slower than BING. Our results therefore suggest that many object proposal methods provide sufficient quality and the choice may be mostly dependent on the speed of the method.

\begin{figure*}[t!]
%   \centering
%   \begin{subfigure}{0.4\textwidth}
%   \centering
%     \includegraphics[width=\linewidth]{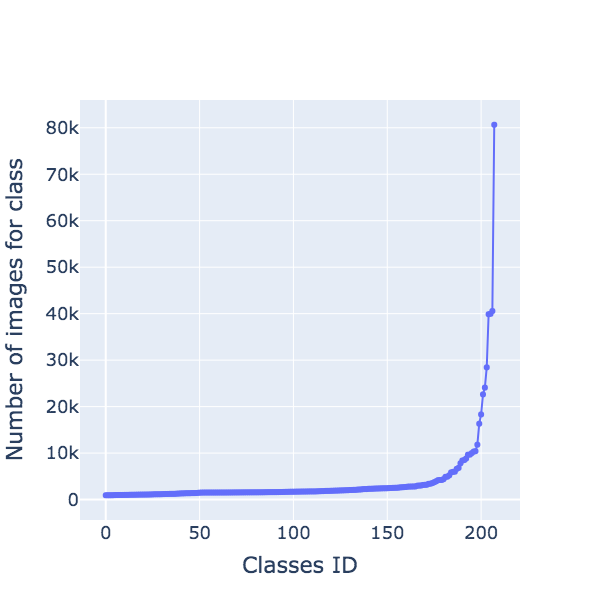}
%     \caption{Distribution of number of images in each class for each of 208 selected classes.}
%      \label{fig:openimages1}
%   \end{subfigure}
%   ~ 
  \begin{subfigure}{0.5\textwidth}
   \centering
    \includegraphics[width=\linewidth]{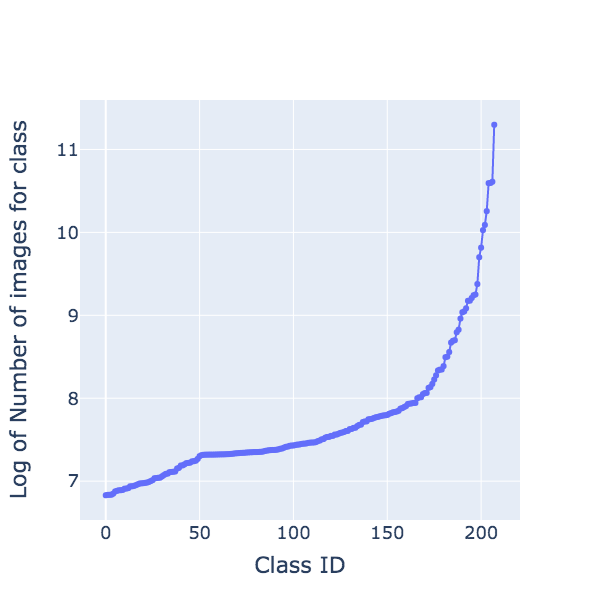}

  \end{subfigure}
  ~
  \begin{subfigure}{0.5\linewidth}
  \centering
    \includegraphics[width=\linewidth]{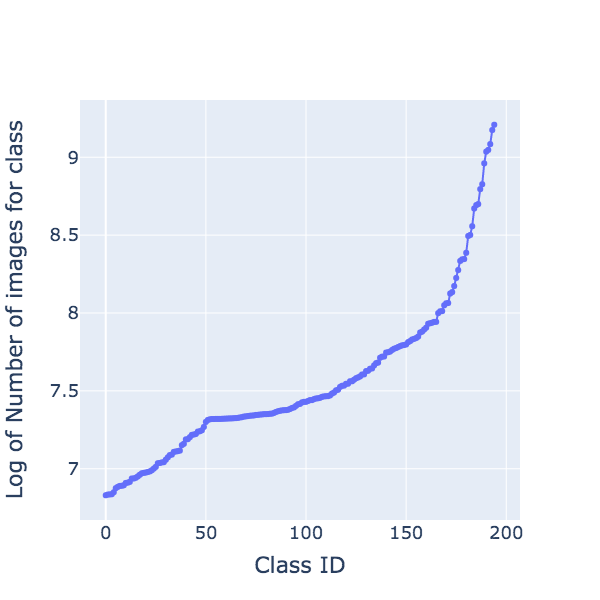}

  \end{subfigure}
  ~
%   \begin{subfigure}{0.5\linewidth}
%   \centering
%     \includegraphics[width=\linewidth]{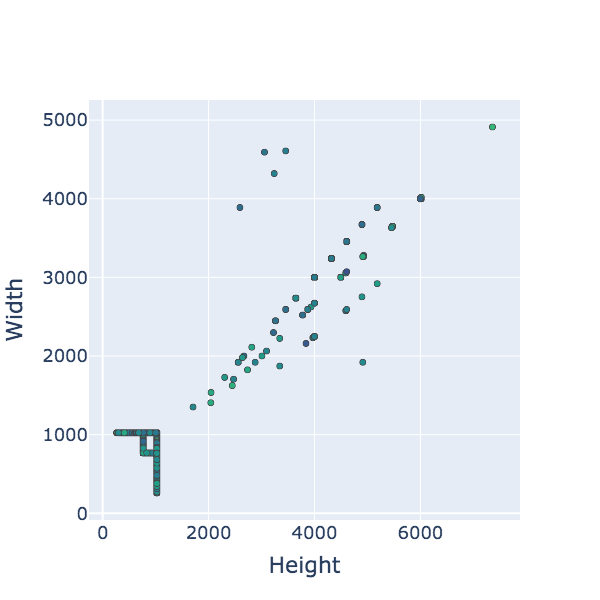}

%   \end{subfigure}
  
  \caption{\textbf{Left:} distribution of number (log) of images in each class for each of 208 selected classes.  \textbf{Right:} scatter plot of the height and width.}
  \label{fig:openimages1_distribution}
  
\end{figure*}

\begin{figure}[t!]
\centering
    \includegraphics[width=0.8\linewidth]{LaTeX/Images/scatter_plot_openimages.png}
    \caption{ Scatter plot of the height and width of the OpenImages Dataset..}
\end{figure}

% In Fig \ref{fig:openimages2} we have removed the classes which had more than 10k images present.
% All of these removed classes are classes such as person, clothing etc which are present in a lot of images. The mean of the number of images per class after removing these classes has come down to 2203.34.

\textbf{(c) Shifted object proposals (Obj-Obj+Shift Crop)}: Unlike Obj-Obj+Dilate, here, the second view is a box selected at random within a pre-specified distance range of the first box (the BING proposal). To choose a pre-specified distance, we choose a random value for the offset from a few ranges: $80$-$100$ pixels; $100$-$120$ pixels etc. 

% Object-Object crop in principle is similar to standard cropping used in SSL approaches like MoCo-v2 \cite{chen2020improved} on ImageNet, since the crops have good amount of overlap with the object.   
% One potential drawback of an object-focused crop is that it ignores context information (scene) which can be useful in disambiguating objects that may be occluded or blurry. 

% \textbf{Value of lower scale of Random-Resized crop for object crops:}
% The Object-Crop usually are not very small and cover a decent portion of the image; on COCO dataset it covers about 39\% of the image and on OpenImages it cover 23\% of the image. So, we instead of using standard scale of 0.2 as the lower scale, we calculate the scale for every dataset. For ex. in case of COCO dataset, since object crops cover 40\% of the image we use 0.4 as the lower scale. Similarly, in case of OpenImages we use 0.2 as the lower scale since object crops cover close to 20\% of the image.
\textbf{(d) Random crop (Obj-Scene Crop):} The first view is the BING proposal; and a regular random crop at scene level is the second view. This method provides information at both object and scene levels, and we use it as a baseline for adding context information to the model. 

\section{More Analysis on OpenImages}
\label{sec:analysis_openimages_more}
\textbf{Varying the temperature parameter}: 
Some self-supervised methods are highly dependent on the temperature hyperparameter, which can can be dataset dependent. The default temp parameter in MoCo-v2 \citep{chen2020improved} (tested on ImageNet) is $0.07$. To ensure that this temperature setting was not a concern for OpenImages, we trained MoCo-v2 models with a number of temperature hyperparameters i.e $0.05, 0.7, 0.1, 0.2$ and $0.3$. We found that a temperature setting of $0.2$ gives the best result which is an increase of $1.2$ mAP over the default value, which is significantly lower than the increase of $8$mAP we get with object cropping. 

\textbf{MoCo-v2 training dynamics:} 
Another potential concern with OpenImages is poor training dynamics of MoCo-v2 on OpenInmages. To verify that this was not the case, we computed the mean inner product positive samples and of negative samples after training MoCo-v2 for $200$ epochs. We find that the mean of the score for positive samples is $0.81$ and the mean of scores of negative samples is $0.005$, very close to the ideal of $1$ and $0$ respectively. This indicates that MoCo-v2 trains properly, and the difference between the MoCo-v2 and supervised training is unlikely to be due to poor training dynamics. 

% \textbf{Random cropping on Ground Truth bounding boxes}: To convert the problem to one similar to ImageNet, we use ground truth bounding boxes and make two random crops on the same object. In essence this will convert the OpenImages dataset to be similar to ImageNet since the majority of images in ImageNet also have one object in an image. However doing so results in very bad performance and can be seen in row1 Table \ref{tab:openimages_analysis}.
% Hence just focusing on the object without taking the context into the account doesn't work quite well. \\

\section{Analysis on Object-Scene crops:}
\label{sec:analysis_object_oobject}

\begin{figure*}[t!]

  \centering
  \begin{subfigure}[t]{0.48\textwidth}
   \centering
    \includegraphics[width=\linewidth]{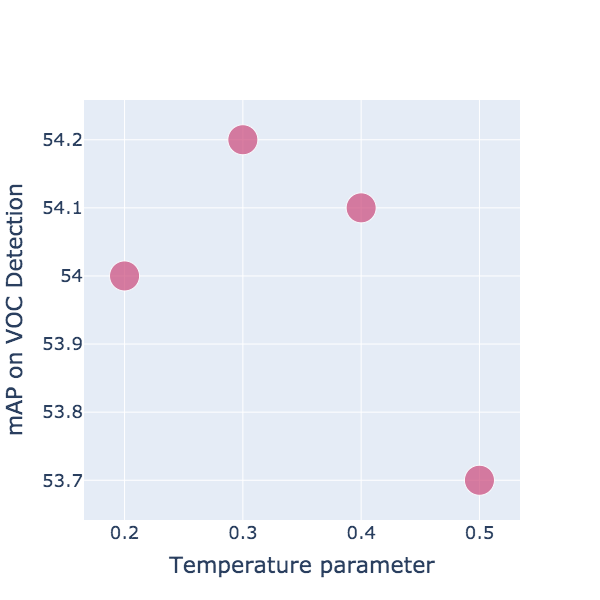}
   
    % \caption{Impact of varying tau.}
     \label{tab:voc_analysis_tau}
  \end{subfigure} 
  ~
  \begin{subfigure}[t]{0.48\linewidth}
   \centering
    \includegraphics[width=\linewidth]{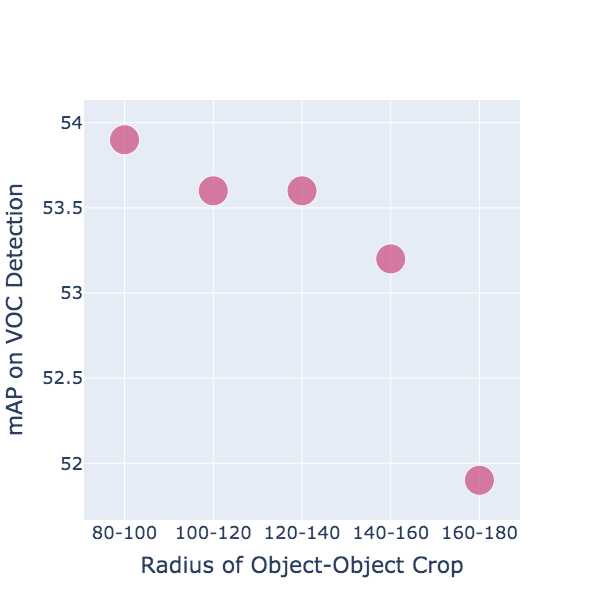}
    % \caption{Impact of varying radius and using all three modalities.}
%   \label{tab:voc_analysis_radius}
  \end{subfigure}

\caption{Results on COCO then transferred to VOC. \textbf{Left}: Varying the temperature parameter.  \textbf{Right}: Varying radius for object-object crop.}
\label{fig:voc_analysis_temp_radius}
\end{figure*}

\begin{figure*}[t!]
  \vspace{-10pt}
  \centering
  \begin{subfigure}[t]{0.48\textwidth}
   \centering
    \includegraphics[width=\linewidth]{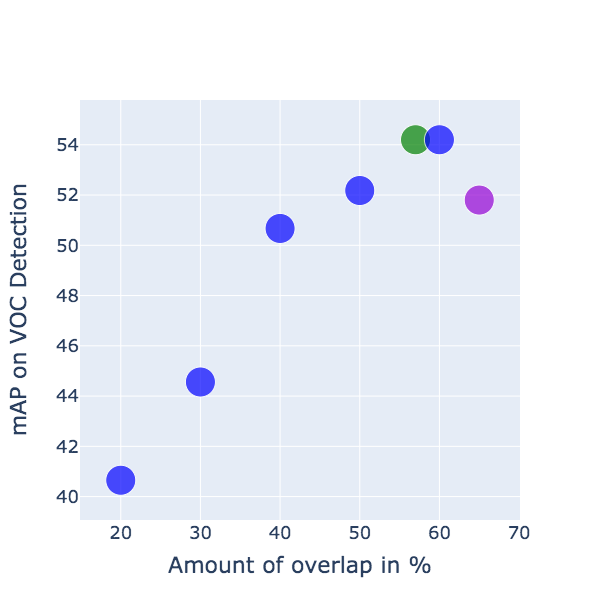}
   
    % \caption{}
     \label{fig:overlap_coco_voc}
  \end{subfigure} 
  ~
  \begin{subfigure}[t]{0.48\linewidth}
   \centering
    \includegraphics[width=\linewidth]{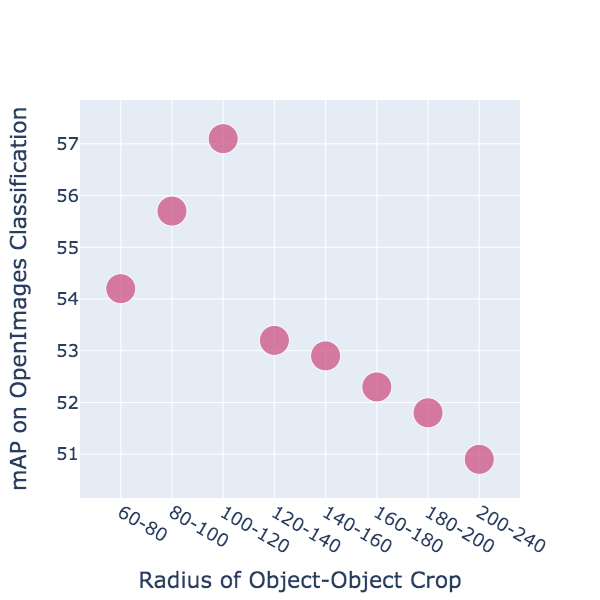}
    % \caption{}
  \label{fig:radius_openimages}
  \end{subfigure}
  \vspace{-0.2in}
    \caption{Left: We vary the amount of overlap between object and scene crops, as shown. Optimal VOC detection performance is achieved around $58\%$ overlap, decreasing on either side. The purple dot indicates overlap for scene-scene crops ($66\%$). Right: We vary the radius of the object-object crops and observe a similar phenomenon of a ``sweet spot" distance between the object crops at which downstream performance is maximized. }
\label{fig:radius_coco_openimages}
\end{figure*}

% \textbf{Analysis of Object-Object crops and Object-Scene crops.}
% We conducted further experiments on iconic datasets and found that using  object-object crops, object-dilated crops and all 3 crops did better than  object-scene (pre-training on COCO; finetuning on the dataset). This implies that, final transfer learning performance is correlated with pretext task. Both the models using context did pretty well on transfer learning tasks which involved predicting multiple objects, like object detection and semantic segmentation, but did poorly on classification on single object datasets. Hence which pre-training methods to use is also dependent on the final downstream tasks. 

% Next, we analyse overlaps in Object-Scene model and Scene-Scene model
% Similarly we analyze the amount of overlap present between Object-Scene crops, and between Scene-Scene crops. We find that between Object-Scene crops there is overlap of 57.23 \% and between Scene-Scene crops overlap is 65.21\% on MS-COCO. Poor performance of random-random can also be attributed to high overlap and the network is not learning good object semantics. 

\textbf{Overlap between crops and object of interest:} In expectation, any two crops of a scene will overlap to some extent. If this intersection overlaps an object, the crops are more likely to contribute to representations that capture object properties.  We measure the fraction of pixels in this intersection that belong to a ground truth object box, to get a sense of how this varies with different cropping strategies and data sets.  We find that this fraction for COCO is $99\%$ for object-scene crops and $92.1\%$ for the scene-scene crop. In the case of OpenImages, the numbers are, respectively, $99.1\%$ and $87.3\%$.  This demonstrates that object-scene crops capture information about objects much more than scene-scene crops, especially in the case of OpenImages.

\textbf{Varying the radius in OpenImages and COCO:} We also vary the radius, which is the distance of the second object-object crop in any random direction from the center of the object crop. We vary this radius under object-object crop when combining all three type of crops. Fig \ref{fig:radius_coco_openimages}(right) shows that, for OpenImages, as we increase the distance of the two object crops, performance first increases and then decreases, again suggesting a sweet spot. We report similar results for COCO dataset in the supplementary.

\textbf{Use of scene information:} To test whether scene information is used by our models, we pre-train two models on the OpenImages dataset: one with object-object cropping and the other with object-scene cropping. Next, we create a new dataset by cropping ground truth bounding boxes from the OpenImages images. Each resulting image contains exactly one object and minimal scene information. We fine-tune the two models on this dataset, and we find that they perform comparably (object-object fine-tuned gives $37$ mAP and object-scene fine-tuned gives $36.4$ mAP). However if we fine-tuned instead on the OpenImages dataset, the object-scene model outperforms by close to $4$ mAP, thus verifying that object-scene model cropping learns features that rely on both object and scene information. \\

\textbf{Varying radius:} Fig. \ref{fig:voc_analysis_temp_radius}(right) shows the performance on VOC (pre-training on COCO) for MoCo-v2 as the radius object-object crops is changed. We see that there is a ``sweet spot" for the radius: neither too large or too small is optimal.

\section{Additional Results}

\textbf{Generating positive samples by randomly cropping on Dilated BING boxes:}
We also try to generate both the positive samples by randomly cropping on the Dilated BING boxes. We find that this method gives us a performance of 54.5 mAP for OpenImages classification. Hence cropping on object boxes and dilated crops are crucial to success of our method.

\textbf{Varying temperature parameter:} We also varied the temperature hyper-parameter for training MoCo-v2 on COCO (transfering to VOC) as seen in Fig. \ref{fig:voc_analysis_temp_radius}(left). We find that temperature of $0.3$ performs best in our setting on the COCO dataset.

\textbf{Varying number of proposals used:} We vary the number of proposals from BING as shown in Table \ref{tab:voc_moco_proposals}. We find that using more proposals results in better performance and we tested upto $10$ proposals per image, finding a consistent boost.

\textbf{Impact of varying scene crop range in the object-scene crop:} We show the effect of varying scene crop range in object-scene crop in Table \ref{tab:openimages_scene_crop_vary}. We can see that as we again reach a sweet spot when the lower crop range is 0.2.

\begin{table*}
    \centering
    \begin{tabu} to \linewidth {lccc} 
        \toprule
        Model & $AP$ & $AP_{50}$ & $AP_{75}$ \\
         \midrule
    %   MoCo-V2 \cite{He2020MomentumCF}  & 50.86 & 77.60&55.43\\
    %     MoCo-V2 using object and context crops (Ours)  & 52.91 & 79.61 & 57.96\\
    Supervised & 56.8 & 83.2 & 63.7 \\
     \midrule
    %Self-EMD \cite{liu2021selfemd}  & 53.0 & 80.0 & 58.6\\
    BYOL Scene-Scene crop \citep{grill2020bootstrap}  & 50.0 & 75.8 & 54.8\\
    MoCo-v2 Scene-Scene crop \citep{chen2020improved}  & 51.8 & 77.6 & 55.4\\
    
    \midrule
    BYOL Obj-Scene crop using BING crops (Ours)  & 52.5 & 77.1 & 58.1\\
    MoCo-v2 Obj-Scene crop using Unsupervised crops (Ours)  & \cellcolor{blue!15} \textbf{53.9} & \cellcolor{blue!15} \textbf{79.8} & \cellcolor{blue!15}\textbf{59.8}\\
    MoCo-v2 Obj-Scene crop using BING crops (Ours)  & \cellcolor{blue!15} \textbf{54.2} & \cellcolor{blue!15} \textbf{80.1} & \cellcolor{blue!15}\textbf{60.0}\\
    MoCo-v2 - Obj-Obj+Dilate  crop ($\delta=0.1$) (Ours) & \cellcolor{blue!15} \textbf{55.0} & \cellcolor{blue!15} \textbf{80.9} & \cellcolor{blue!15}\textbf{60.7}\\
    \midrule
    Dene-CL \citep{wang2021dense}  & 56.7 & 82.5 & 63.8\\
    Dense-CL with Obj-Obj+Dilate crop (Ours)  & \cellcolor{blue!15} \textbf{57.6} & \cellcolor{blue!15} \textbf{82.5} & \cellcolor{blue!15}\textbf{63.8}\\
        \bottomrule
    \end{tabu}
    \caption{Object detection results on VOC dataset (COCO pre-training). All models have been pre-trained on COCO and then fine-tuned on VOC. For both MoCo-v2 and BYOL, replacing the default scene crops with object-scene crops results in a consistent improvement. }
    \label{tab:voc_moco}
    
\end{table*}

\begin{table*}
    \centering
    \begin{tabu} to \linewidth {lccc} 
        \toprule
        Model & $AP$ & $AP_{50}$ & $AP_{75}$ \\
         \midrule
    %   MoCo-V2 \cite{He2020MomentumCF}  & 50.86 & 77.60&55.43\\
    %     MoCo-V2 using object and context crops (Ours)  & 52.91 & 79.61 & 57.96\\
    Supervised & 56.8 & 83.2 & 63.7 \\
     \midrule
    %Self-EMD \cite{liu2021selfemd}  & 53.0 & 80.0 & 58.6\\
    Baseline (Scene-Scene)	 \citep{chen2020improved}  & 51.5 & 79.4 & 56.1\\
    Ours (Obj-Scene)	 \citep{chen2020improved}  & 53.0 & 79.3 & 58.3\\

        \bottomrule
    \end{tabu}
    \caption{Object detection results on VOC dataset (OpenImages pre-training). All models have been pre-trained on OpenImages and then fine-tuned on VOC.  Replacing the default scene crops with Obj-Scene crops results in a consistent improvement. }
    \label{tab:voc_moco_openimages}
    
\end{table*}

\begin{table*}
    \centering
    \begin{tabu} to \linewidth {lcccc} 
        \toprule
        Model & Proposals  & $AP$ & $AP_{50}$ & $AP_{75}$ \\
         \midrule
    %   MoCo-V2 \cite{He2020MomentumCF}  & 50.86 & 77.60&55.43\\
    %     MoCo-V2 using object and context crops (Ours)  & 52.91 & 79.61 & 57.96\\
    Supervised & - & 56.8 & 83.2 & 63.7 \\
     \midrule
    %Self-EMD \cite{liu2021selfemd}  & 53.0 & 80.0 & 58.6\\
    
    MoCo-v2 Obj-Scene crop \citep{chen2020improved}  & 1 & 51.9 & 77.6 & 55.4\\
    MoCo-v2 Obj-Scene crop \citep{chen2020improved}  & 5 & 53.5 & 79.4 & 56.4\\
    
    MoCo-v2 Obj-Scene crops using BING crop (Ours)  & 10& \cellcolor{blue!15} \textbf{54.2} & \cellcolor{blue!15} \textbf{80.1} & \cellcolor{blue!15}\textbf{60.0}\\
        \bottomrule
    \end{tabu}
    \caption{Varying the number of proposals generated by BING. All models are pre-trained on COCO and then fine-tuned on VOC Object Detection. Increasing the number of proposals provides a consistent boost. We used $10$ proposals as this was close to the average number of objects per image in OpenImages.}
    \label{tab:voc_moco_proposals}
    
\end{table*}

\begin{table*}
    \centering
    \begin{tabu} to \linewidth {lcccc} 
        \toprule
        Model & $\delta$  & $AP$ & $AP_{50}$ & $AP_{75}$ \\
         
     \midrule
    %Self-EMD \cite{liu2021selfemd}  & 53.0 & 80.0 & 58.6\\
    
    MoCo-v2 & 0 & 54.3 & 77.1 & 5484\\
    MoCo-v2  & 0.1 & 55.1 & 81.0 & 60.7\\
    MoCo-v2 & 0.2 & 54.5 & 80.7 & 60.3\\
    MoCo-v2 & 0.3 & 54.2 & 80.2 & 60.1\\
    
        \bottomrule
    \end{tabu}
    \caption{Varying dilation i.e $\delta$ on the COCO dataset for Obj-Obj+Dilate crop strategy. All models have been pre-trained on COCO and then fine-tuned on VOC Object Detection. $\delta=0$ corresponds to Obj-Obj cropping and larger $\delta$ is very similar to Obj-Scene. A sweet spot exists between the extremes.}
    \label{tab:dilation_vary_coco}
    
\end{table*}

\begin{table}
    \centering
    \begin{tabu} to \linewidth {lccc} 
        \toprule
        Dataset & Obj-Scene (Top-1)  & Obj-Obj+Dilate (Top-1) \\

         \midrule
       %Ground truth object crops & 22.8 \\
    %   Aircraft	& 87.8 &	88.7  & 88.7 \\
    %   Stanford Cars	& 89.1 &	90.7  & 90.7  \\
    %   Caltech-UCSD Birds	& 87.2 &88.8  & 88.8 \\
       Aircraft	& 87.8 &	88.7 \\
      Stanford Cars	& 89.1 &	90.7   \\
      Caltech-UCSD Birds	& 87.2 &88.8\\
        \bottomrule
    \end{tabu}
    \vspace{0.1in}
    \caption{Obj-Obj+Dilate crop pre-training consistently outperforms Obj-Scene for transfer to various downsteam datasets for classification (COCO pre-training).}
    % \vspace{-1.5ex}
    \label{tab:object-object-analysis}
\end{table}

\begin{table*}
    \centering
    \begin{tabu} to \linewidth {lccc} 
        \toprule
        Model & mAP (Classification) \\
         \midrule
         Supervised OpenImages & 66.3
        \\ 
         \midrule
       %Ground truth object crops & 22.8 \\
       
       MoCo-v2: Scene Crop Range (Object-Scene) $0.8$-$1.0$ & 34.2 \\
       MoCo-v2: Scene Crop Range (Object-Scene) $0.6$-$1.0$ & 46.1 \\
       MoCo-v2: Scene Crop Range (Object-Scene) $0.4$-$1.0$ & 54.3 \\
       MoCo-v2: Scene Crop Range (Object-Scene) $0.2$-$1.0$ & 58.1 \\
       MoCo-v2: Scene Crop Range (Object-Scene) $0.1$-$1.0$ & 56.3 \\
       MoCo-v2: Scene Crop Range (Object-Scene) $0.05$-$1.0$ & 53.5 \\
        \bottomrule
    \end{tabu}
    \vspace{0.1in}
    \caption{Impact of varying scene crop range in the object-scene crop.}
    % \vspace{-1.5ex}
    \label{tab:openimages_scene_crop_vary}
\end{table*}

\textbf{Results after 200 epochs training:} We show results after training 200 epochs of training in Table \ref{tab:voc_moco_200}. We compare these results with 800 epochs and we can see their a good co-relation between results after 200 epochs and after 800 epochs. This could be useful in low compute regime  settings, since training 200 epochs is highly indicative of performance after longer training schedules.

\begin{table*}
    \centering
    \begin{tabu} to \linewidth {lccccccc} 
        \toprule
         Description & epochs & $AP$ & $AP_{50}$ & $AP_{75}$ & $AP_{s}$ & $AP_{l}$ & $AP_{m}$ \\
         \midrule
    MoCo-v2 Scene-Scene crop  & 200  & 34.6 & 53.5 & 37.0 & 30.4 & 50.1 & 32.3\\
    
    MoCo-v2 Obj-scene crop (Ours)   &200 & \cellcolor{blue!15} \textbf{35.6} & \cellcolor{blue!15} \textbf{54.3} & \cellcolor{blue!15}\textbf{38.3} & \cellcolor{blue!15} \textbf{31.3} & \cellcolor{blue!15}\textbf{51.2}
    &\cellcolor{blue!15}\textbf{33.4}\\
    \midrule
    MoCo-v2 & 800 & 38.2 & 58.9 & 41.6 & 34.8 & 55.3 & 37.8\\
     MoCo-v2 Obj-Scene crop (Ours)& 800  & \cellcolor{blue!15}\textbf{39.4} & \cellcolor{blue!15}\textbf{59.8} & \cellcolor{blue!15}\textbf{42.9} & \cellcolor{blue!15}\textbf{35.8} & \cellcolor{blue!15}\textbf{57.8} & \cellcolor{blue!15}\textbf{38.7}\\
        \bottomrule
    \end{tabu}
    \caption{Results after pre-training for 200 epochs. These results are highly indicative of results we get after longer training and can be useful for comparison in less compute settings.}
    \label{tab:voc_moco_200}
    
\end{table*}

% \subsection{Results of longer pre-training:} 
% We also results of longer pre-training.

\section{Visualizations}
We show additional examples of object crops and scene (random) crops in Figures \ref{tab:viz_bing1}, \ref{tab:viz_bing2}, \ref{tab:viz_bing3}, \ref{tab:viz_bing4}, \ref{tab:viz_bing5}. We can see in all these images random scene crops often miss out objects of interest while BING tends to capture them. We also show visual comparison between OpenImages and ImageNet as shown in Fig \ref{fig:imagenet_openimages_figure}. We can see that ImageNet images are centered and mostly occupy the center part of the image, which is not the case with OpenImages.

\begin{figure*}[t!]

  \centering
%   \begin{subfigure}[t]{\textwidth}
   \centering
    \includegraphics[width=\linewidth]{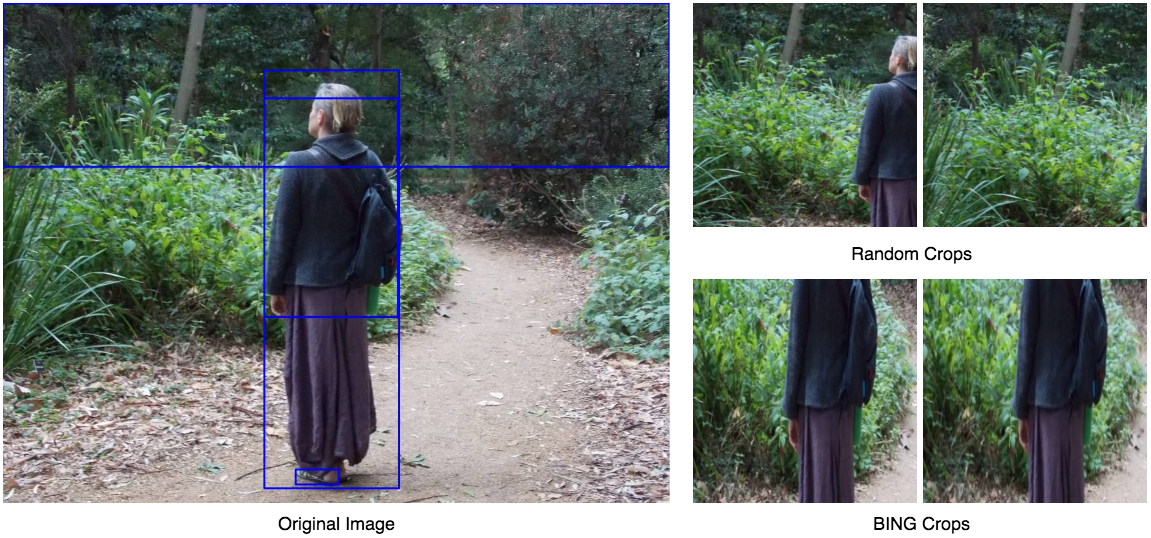}
   
    \caption{Visualization of BING and random crops. }
     \label{tab:viz_bing1}
%   \end{subfigure} 
\end{figure*}

\begin{figure*}[t!]

  \centering
%   \begin{subfigure}[t]{\textwidth}
   \centering
    \includegraphics[width=\linewidth]{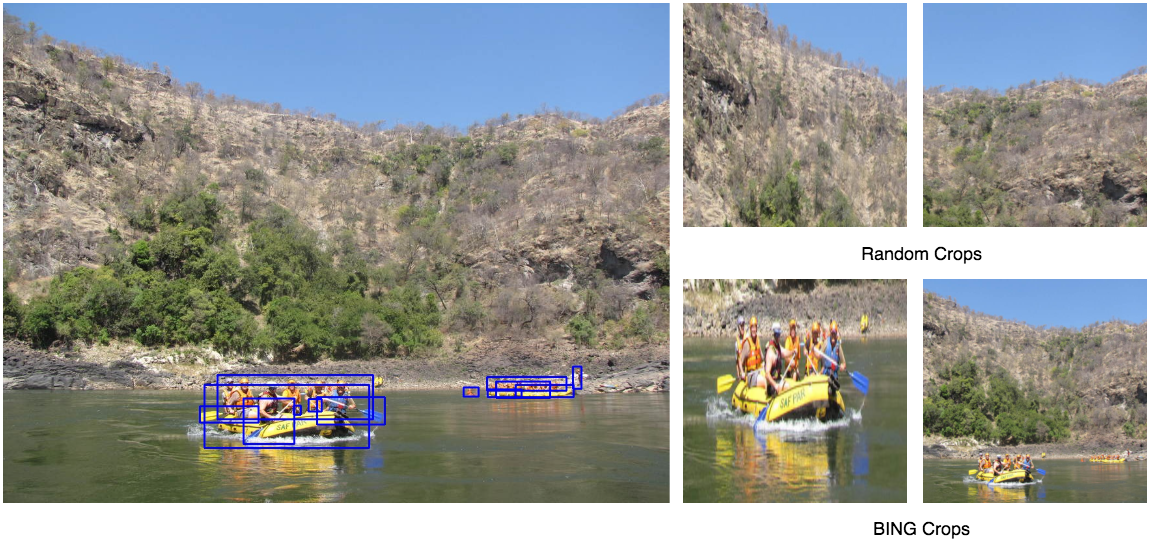}
   
    \caption{Visualization of BING and random crops.}
     \label{tab:viz_bing2}
%   \end{subfigure} 
\end{figure*}
\begin{figure*}[t!]

  \centering
%   \begin{subfigure}[t]{\textwidth}
   \centering
    \includegraphics[width=\linewidth]{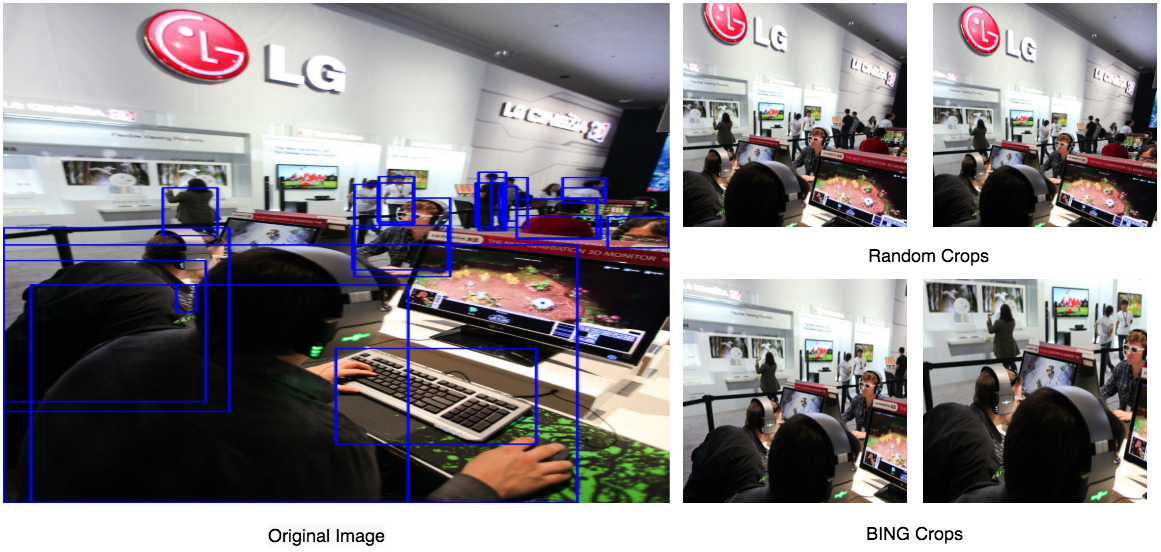}
   
    \caption{Visualization of BING and random crops.}
     \label{tab:viz_bing3}
%   \end{subfigure} 
\end{figure*}
\begin{figure*}[t!]

  \centering
%   \begin{subfigure}[t]{\textwidth}
   \centering
    \includegraphics[width=\linewidth]{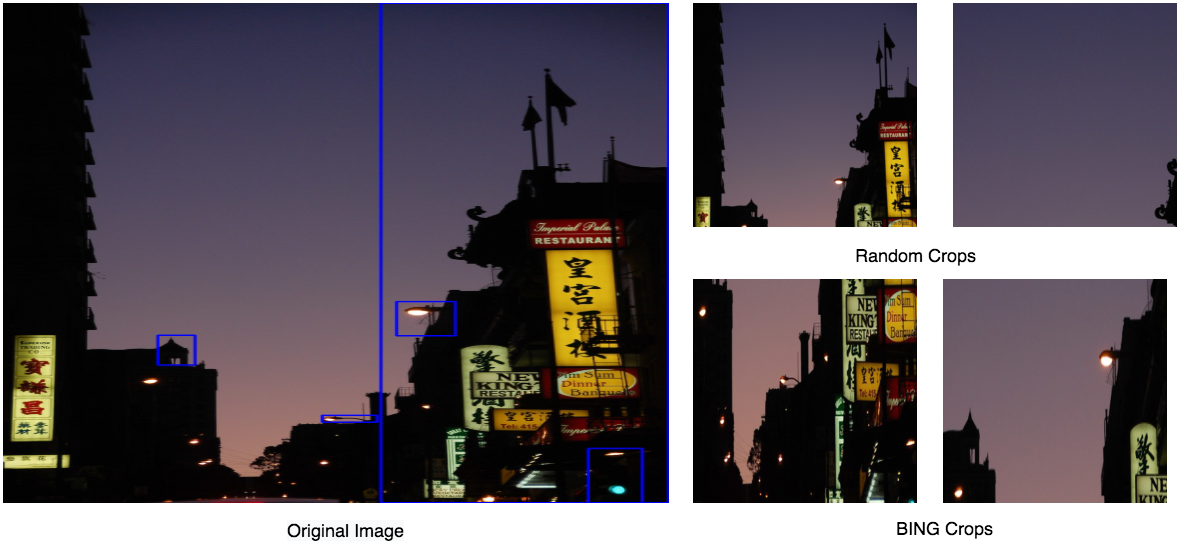}
   
    \caption{Visualization of BING and random crops.}
     \label{tab:viz_bing4}
%   \end{subfigure} 
\end{figure*}
\begin{figure*}[t!]

  \centering
%   \begin{subfigure}[t]{\textwidth}
   \centering
    \includegraphics[width=\linewidth]{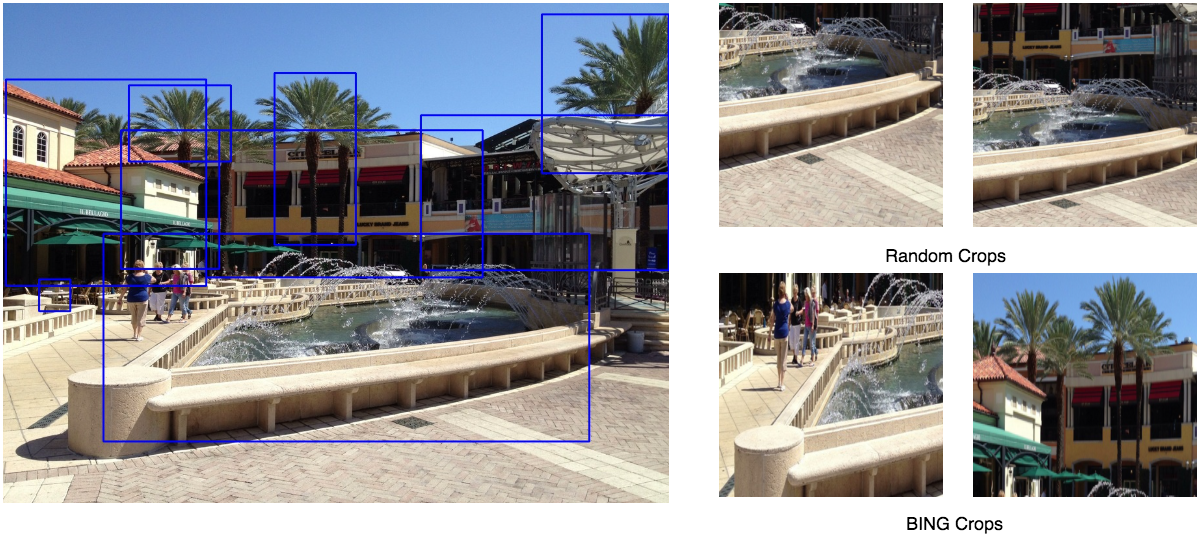}
   
    \caption{Visualization of BING and random crops.}
     \label{tab:viz_bing5}
%   \end{subfigure} 
\end{figure*}

\begin{figure*}[h!]
  \centering
  \begin{subfigure}{\linewidth}
    \includegraphics[width=\linewidth]{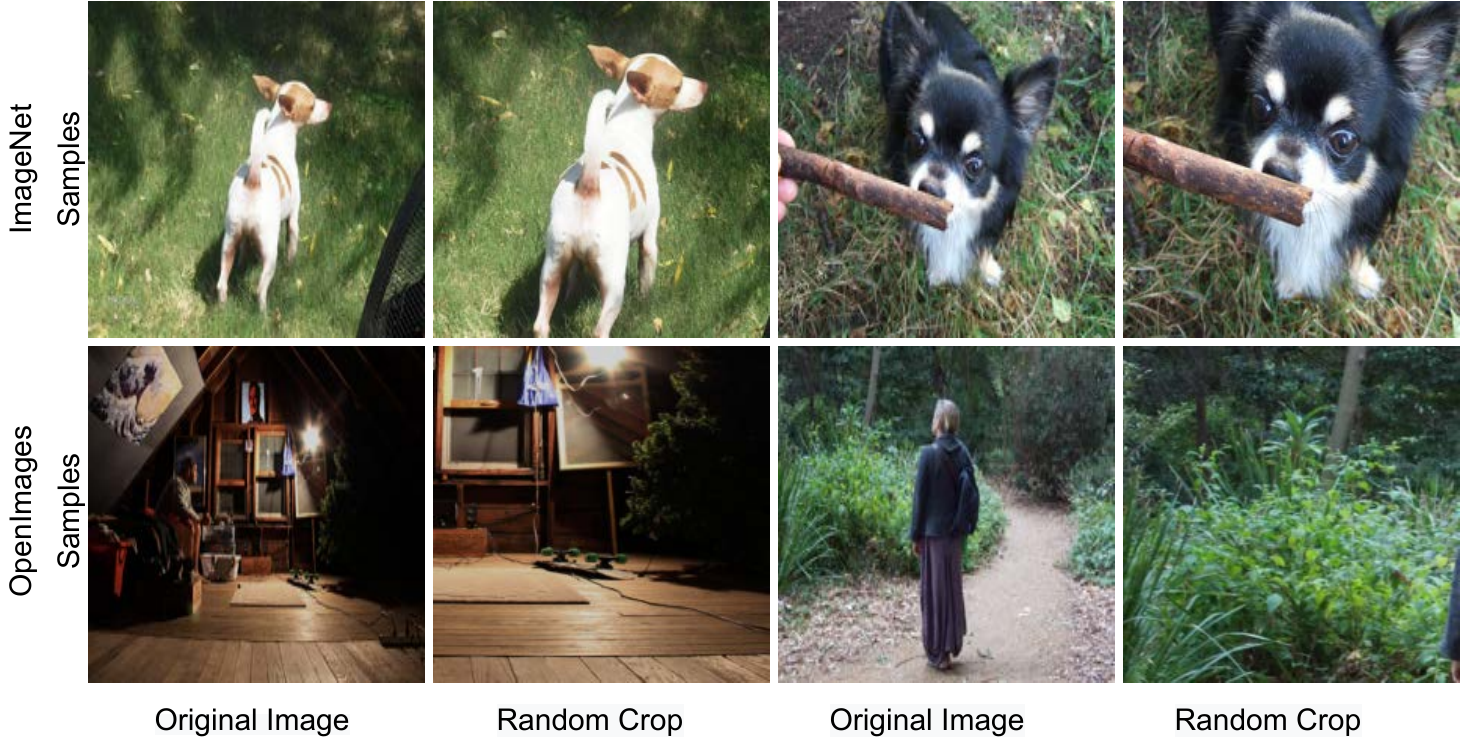}
  \end{subfigure}
  \caption{First column: Two samples from OpenImages dataset. Second and Third Columns: Random scene crops; Fourth and fifth columns: Random object crops generated by the BING \citep{Cheng2014BINGBN} algorithm. We see that the object crop tends to center on objects in the image that are often missed by the scene crops.}
  \label{fig:imagenet_openimages_figure}
\end{figure*}

\begin{table*}
    \centering
    \begin{tabu} to \linewidth {lcccccc} 
        \toprule
        Description & $AP$ & $AP_{50}$ & $AP_{75}$ & $AP_{s}$ & $AP_{l}$ & $AP_{m}$\\
        
    %   MoCo-V2 \cite{He2020MomentumCF}  & 50.86 & 77.60&55.43\\
    %     MoCo-V2 using object and context crops (Ours)  & 52.91 & 79.61 & 57.96\\
    
     \midrule
    MoCo-v2 & 39.8 & 59.8 & 43.6 & 36.1 & 56.9 & 38.7\\

    MoCo-v2 (Obj-Obj+Dilate $\delta=0$) (Ours)  & \cellcolor{blue!15}\textbf{40.2} & \cellcolor{blue!15}\textbf{60.6} & \cellcolor{blue!15}\textbf{43.6} & \cellcolor{blue!15}\textbf{36.4} & \cellcolor{blue!15}\textbf{57.4} & \cellcolor{blue!15}\textbf{39.0}\\
    \midrule
    MoCo-v2 &  57.0 & 82.2 & 63.4 & - & - & -\\
    MoCo-v2 (Obj-Obj+Dilate $\delta=0$) & \cellcolor{blue!15} \textbf{57.8} & \cellcolor{blue!15} \textbf{82.9} & \cellcolor{blue!15}\textbf{64.2} & - & - & -\\
        \bottomrule
    \end{tabu}
    \caption{Object detection results on COCO (top 2 rows) and VOC (bottom 2 rows). All SSL models have been pre-trained on ImageNet for 200 epochs and then fine-tuned on COCO and VOC.}
    \label{tab:imagenet_results}
\end{table*}

\section{Implementation Details}
We use a ResNet-50 \cite{He2015} deep network as the backbone for all experiments. After pre-training, we freeze the backbone weights, and train a linear classifier or fine-tune on the downstream datasets and tasks. We also train a randomly initialized ResNet-50 network in a fully supervised manner using ground truth labels and a multi-class logistic regression loss. We follow the mAP metric as described in section 4.2 of paper \cite{veit2017learning} (Eqn.(4)).

One additional change that we make to object crops is if the size of the object proposal is small, i.e less than 224$\times$224, we use a larger crop from the original image so that the size of the crop is at least 224$\times$224. To achieve this, we pick the center of the object-crop in the original image and cut a center crop of size 224$\times$224 from original object-crop center. Hence the object-crops for images smaller than 224$\times$224 are not tight bounding boxes but bigger crops with objects in it. Additionaly we find that $delta$ = $0.1$ works well for COCO and  $delta$ = $0.2$ works well for OpenImages.

{We randomly choose one of scene or object to pass through the query & key encoder. Thus, either the “scene” or “object” crop could be the “teacher”. 2) Different from the standard contrastive learning setup, we train two (query) MLPs , one each for object and scene crop and maintain EMA versions of the two on the student (key) side.} 

\subsection{Hyperparameters for different methods}
We train all the SSL methods for 200 epochs on OpenImages-Subset unless mentioned otherwise. 

\textbf{MoCo-v2:} For MoCo-v2 \citep{chen2020improved} we closely follow the standard hyper-parameters (given in the main paper). We used a learning rate of $0.03$ using SGD as our optimizer, weight decay of $10^{-4}$ and initial learning rate of $0.03$. To traine OpenImages-Subset, we trained for 200 epochs and for COCO, following DenseCL \citep{wang2021dense}, we trained for 800 epochs.

\textbf{Supervised Training on OpenImages:} For supervised training on OpenImages, we use standard Adam optimizer with learning rate of $10^{-3}$, patience of 5 epochs and trained the network for $90$ epochs. 

\textbf{CMC:} We follow the standard hyperparameters following CMC\citep{tian2019contrastive}: temperature $0.07$, momentum $0.5$ and learning rate $0.03$. 

\textbf{BYOL:} For BYOL, we used LARS optimizer with learning rate of $0.2$, following the standard hyperparameters listed in \citep{grill2020bootstrap}. 

\textbf{SWaV:} For SWaV the standard hyperparameters listed in SWaV \citep{NEURIPS2020_70feb62b} do not work well for OpenImages-Subset (the authors do not show results on this dataset in their paper). So following their FAQ's in the offical github repositry (\url{https://github.com/facebookresearch/swav}) we tried few different hyperparameters. Intially we started with epsilon of 0.05 and then decreased it to 0.03. We also deceased the LR to half and froze the prototypes during the first few iterations. We trained to network for 200 epochs.

{\subsection{Computational cost of running LOD:}
For OHMS, it took around 4.5 hrs to generate the proposals and for COCO it took us ~2 hours to generate the proposals.}

% \subsection{Other details on cropping}
% One additional change that we make to object crops is if the size of the object proposal is small i.e less than 224*224, we use a larger crop from the original image so that the size of the crop is at least 224*224. To achieve this, we pick the center of the object-crop and in the original image and cut a center crop of size 224*224 from original object-crop center. 

% \begin{figure*}[h!]
%   \centering
%   \begin{subfigure}{\linewidth}
%     \includegraphics[width=\linewidth]{LaTeX/Images/2bing_2open_1.png}
%   \end{subfigure}
%   \caption{First column: Two samples from OpenImages dataset. Second and Third Columns: Random scene crops; Fourth and fifth columns: Random object crops generated by the BING \citep{Cheng2014BINGBN} algorithm. We see that the object crop tends to center on objects in the image that are often missed by the scene crops.}
%   \label{fig:figure_openimages_vis}
% \end{figure*}
\section{Theoretical motivation}
Our hypothesis is that uniformly random image cropping has a high likelihood of missing relevant objects or having other noisy signals. This is especially true when objects are small relative to the size of the image. This leads to suboptimal representations for multi-object datasets such as OpenImages due to the inclusion of data that is weakly correlated with the objects of interest. To overcome this, we propose using semantic information in the cropping to ensure a higher probability of selecting crops around relevant  semantic objects in the scene. While we apply our techniques to several self-supervised training approaches, our intuition is best understood in the context of contrastive learning frameworks.  

It has been shown\citep{Oord2018RepresentationLW} that objectives such as InfoNCE estimate a lower bound on $I(X;C)$, where I(.;.) is the mutual information, $X$ is the  "image signal of interest" ($X$) and the correlated context ($C$). InfoNCE approximates the lower bound by maximizing the correlation between encoded image inputs $g_\theta(X)$ and $g_\theta(C)$,  while using uncorrelated contexts to prevent code collapse. Here $g_\theta$ is the neural network parameterized by $\theta$, and $\theta$ is optimized using stochastic gradient descent based optimization. 

% We can rephrase it so that we now plug in both p'(x) and p'(c|x). So we can say that object-object crops are also an instance of our plug-in procedure. 
$I(X;C)$ can be rewritten as $\int_{x,c} p(x,c) \log (p(x|c)/ p(x))dxdc$ . The statement for our approach is that \emph{we plug in a new p'(x) that concentrates the probability mass around regions of $X$ that are strongly correlated with artefacts of interest in the downstream tasks}. Intuitively, this ensures that the training procedure for $g_\theta$ is more focused on $X$ samples that are strongly correlated with objects of interest.  For downstream tasks such as object recognition and detection, we can approximate "strong correlation with artefacts of interest" in a crop with the presence of objects in that crop. Therefore our approach can be interpreted as plugging in a new distribution p'(x) in the place of p(x) in the following InfoNCE equation. 

\begin{equation}
I(X;C) =\int_{x,c} p(x,c) \log \frac{p(x|c)}{ p(x)}dxdc \geq   \int_{(x,c,c'_{1:k})} -\log \frac{f(x,c)}{f(x,c)+ \sum_k f(x,c'_k)} d(x,c,c'_{1:k})
\end{equation}

%fill in the expression later ( Abhyuday)
Here $f$ is the function used to compute the density ratio \citep{Oord2018RepresentationLW} and $c'_{1:k}$ are the $k$ negative samples. 
Our proposed p'(x) should produce a set of samples that are more enriched with object-centric crops. To produce this enriched sample set,  we use three object proposal models: BING \citep{Cheng2014BINGBN} and Edge-Boxes \citep{Zitnick2014EdgeBL}, both of which are trained with boxes from Pascal-VOC; and an unsupervised object proposal method \citep{vo2019unsupervised}. {Note that P’(x) results from the new sampling scheme defined by our proposed cropping methods. So each of our cropping scheme can be viewed as enforcing a different probability distribution over x in (1).}

In the later sections of this paper, we provide experimental result that validate the hypothesis that our plugged in p'(x) distribution leads to improved downstream performance. Additionally, our schema also shows improvement over self-supervised approaches, such as BYOL and self-EMD, which cannot be decomposed into a gradient descent procedure for an objective function. Our approach also seems to complement methods like self-EMD that are already designed to improve performance on non-iconic image datasets such as COCO.
\textbf{Analysis of Obj-Scene and Obj-Obj+Shift crops:} As shown in \cite{tian2019contrastive}, the performance of contrastive self-supervised methods is have ``sweet spot" which correspond to an optimal amount of MI between views. We perform a similar analysis on the Obj-Scene crop approach by creating crops with progressively higher overlaps. Fig.\ref{fig:radius_coco_openimages}(left) (supplementary) shows the performance peaks around an overlap of $57.2\%$. This finding is consistent with that of \cite{tian2019contrastive}. Scene-Scene crop has a higher optimal overlap of $65.2\%$. Varying the radius of Obj-Obj+Shift crop (Fig \ref{fig:radius_coco_openimages}(right) for OHMS; Fig.\ref{fig:voc_analysis_temp_radius}(right) for COCO shows similar results. We show additional analysis on overlap between crops and object of interest in Section \ref{sec:analysis_object_oobject}. 
